# Supplementary material for: NaVid: Video-based VLM Plans the Next Step for Vision-and-Language Navigation
Source: arXiv:2402.15852 source file (2024-06-30)
Supplement: Supplementary file 1 [file main_suppl.tex]

\documentclass[conference]{IEEEtran}
\usepackage{times}

% numbers option provides compact numerical references in the text. 
\usepackage[numbers]{natbib}
\usepackage{multicol}
\usepackage{balance}
\usepackage[bookmarks=true]{hyperref}
\usepackage{flushend}

% added by Rongtao
\usepackage{xcolor}

% added by Zhizheng
\usepackage{tcolorbox}

 %there is no space
 %there is no space
 %there is no "."

\pdfinfo{
   /Author (Homer Simpson)
   /Title  (Robots: Our new overlords)
   /CreationDate (D:20101201120000)
   /Subject (Robots)
   /Keywords (Robots;Overlords)
}

\input{ourcommands}

\begin{document}

% paper title
% \title{NaviVLM: Vision Language Model for Vision Language Navigation by Encoding Monocular Video Input}
%\title{NaVid: Video-Language Model Plans the Next Step\\ for Vision-and-Language Navigation} %Zhizheng
\title{Supplemental Material of NaVid} %Zhizheng

\maketitle

\IEEEpeerreviewmaketitle

\input{paper/suppl}

\bibliographystyle{plainnat}
\bibliography{references}

\end{document}
